# Supplementary material for: Lite2Relight: 3D-aware Single Image Portrait Relighting
Source: arXiv:2407.10487 source file (2024-07-15)
Supplement: Supplementary file 1 [file 06_supp.tex]

\section{Implementation Details}
\label{sec:implementation_details}

\subsection{ Training and Testing Details}
% We implement our $\latentNet$ in Pytorch \cite{torch}. Our $\latentNet$ consists of 14 MLP layers with ReLU activation and optimizes the objective functions defined in Sec 3.4. We use Adam optimizer~\cite{KingBa15} at a learning rate of $0.0003$ and use weight of $\wtl=10, \wtc=0.01, \wtp=1.0$ for the $\lossl$ $\lossc$ and $\lossp$ losses respectively.
% %
% We use the pretrained checkpoints of the EG3D, $\encoder$, and $\afa$ from the original implementations. 
% %
% We train our method on images of 250 subjects from two frontal viewpoints, where each subject is relit under 50 random natural illumination conditions.
% %
% Our entire training takes about 16 hours on two A100/A40 GPUs for 27k iterations with a batch size of 8.

% Given a monocular image during test time, our approach takes about $140 ms$ to invert and relight. After embedding the subject in the, for a given target illumination, we can render novel viewpoints at 31 frames per second on an A40 GPU.

We implemented our method using PyTorch \cite{torch}. $\latentNet$ comprises 14 MLP layers with ReLU activations. It is designed to optimize the objective functions detailed in Sec 3.4. For optimization, we employ the Adam optimizer~\cite{KingBa15} with a learning rate of $0.0003$. The weights for the losses $\lossl$, $\lossc$, and $\lossp$ are set at $\wtl=10, \wtc=0.01, \wtp=1.0$, respectively.

We utilize the pretrained checkpoints of EG3D, $\encoder$, and $\afa$ from their original implementations. Our training dataset includes images of 250 subjects captured from two frontal viewpoints, each subject being relit under 50 different natural illumination conditions.

The entire training process is completed in approximately 16 hours over two A100/A40 GPUs. This is achieved across 27k iterations with a batch size of 8.

In a testing scenario with a monocular image, our approach requires around $140 ms$ for inversion and relighting. Once the subject is embedded in the target illumination environment, we can render novel viewpoints at a rate of 31 frames per second on an NVIDIA A40 GPU.

\subsection{Interactive Demo Details}
\input{tex_fig/results/supmat_demo}
% We additionally demonstrate the effectiveness of \OurMethod through a user demo driven from a web camera on a workstation with a single NVIDIA 3090 GPU.
% Currently, our demo involves live tracking and alignment of the user's head using face landmarks. Then at every frame, through a single forward pass, we invert the subject and load the desired environment map and render at novel viewpoints and relight on the fly as shown in the \cref{fig:challenges}. Currently, our demo runs at 7 frames per second, and we want to bring to the attention of the readers that though further engineering optimizations we can improve the runtime performance of our demo. Further, we provide additional video demonstration of our user demo in the supplemental videos. 

% In addition to our technical evaluations, we showcase the practical effectiveness of \OurMethod with a user demo, powered by a web camera on a workstation equipped with a single NVIDIA 3090 GPU. This live demonstration involves real-time tracking and alignment of the user's head using facial landmarks. For each frame, our method efficiently inverts the subject, applies the selected environment map, and performs relighting and viewpoint rendering dynamically, as illustrated in \cref{fig:demo}. Currently, our demo operates at a rate of 7 frames per second. We wish to highlight that with further engineering and optimization, there is good potential to enhance the runtime performance of our demonstration.

% Additionally, we provide a comprehensive video showcasing the capabilities of our user demo in the supplementary materials.

In addition to our technical evaluations, we showcase the practical effectiveness of \OurMethod with a user demo, powered by a web camera on a workstation equipped with a single NVIDIA 3090 GPU. This live demonstration involves real-time tracking and alignment of the user's head using facial landmarks. For each frame, our method efficiently inverts the subject, applies the selected environment map, and performs relighting and viewpoint rendering dynamically, as illustrated in \cref{fig:demo}. Currently, our demo operates at a rate of 7 frames per second. We wish to highlight that with further engineering and optimization, there is significant potential to enhance the runtime performance of our demonstration.

Additionally, we provide a comprehensive video showcasing the capabilities of our user demo in the supplementary materials. This video aims to give viewers a more tangible sense of the real-time interactivity and effectiveness of \OurMethod in a live setting.

\section{Ablation Study}~\label{subsec:results_ablation}

\paragraph{Additional Evaluation Metrics:}~\label{abln_additional_metrics}
\new{To further emphasize on quality of relighting, we provide additional evaluation metrics such as LPIPS~\cite{justin_percetptual_loss}, RMSE and DISTS~\cite{ding2020iqa} loss metrics. We observe that \OurMethod convincigly outperfroms the baseline methods as shown in \cref{tab:abln_additional_metrics}.}
\begin{table}[ht]
\centering
\caption{\textbf{Quantitative Results: Ablation Study: Additional Metrics.} We report LPIPS, RMSE and DISTS metrics in addition to SSIM, landmarks distance (LD), and PSNR on the test data of lightstage, where  subjects are relit under novel viewpoints.} 
\begin{tabular}{lcccccc}
\hline 
           & LPIPS$\downarrow$ & RMSE$\downarrow$ & DISTS$\downarrow$  \\ \hline
PhotoaApp  & 0.4163 & 0.1988 & 0.2031  \\
NeRFFaceLighting & 0.2966 & 0.2905 & 0.2409  \\ \hline
\OurMethod &  \textbf{0.2493}& \textbf{0.1841} & \textbf{0.1718} \\ \hline
\end{tabular}
\label{tab:abln_additional_metrics}
\end{table}

% \new{
% \paragraph{NeLF} NeLF requires at least three input views to obtain reasonable results. This makes NeLF unusable for almost all in-the-wild portraits. Moreover, NeLF struggles to reconstruct a reasonable facial structure even with multiview inputs as it fails to represent the underlying geometry leading to low scores in \cref{tab:baseline-single_view}.
%  We can observe the results in \cref{fig:ours_vs_nelf}, where NeLF's results were obtained from 3 input views producing distorted facial reconstructions. In contrast, our approach demonstrates superior generalization to novel subjects from a single image. Furthermore, our method exhibits the ability to accurately relight these subjects, maintaining both the integrity of facial features and the overall photorealism.}
%
\paragraph{Number of Viewpoints: }~\label{abln_subsec_n_views}
As our 3D face prior was derived from monocular data, we delved into examining the necessity of multiple viewpoints in the training of our relighting network, $\latentNet$.
To this end, we trained various iterations of $\latentNet$ using different sets of viewpoints—specifically, 1, 2, 4, and 8 viewpoints. The outcomes of these experiments are systematically presented in ~\cref{tab:abln_n_views}. A noteworthy observation from our study is the robustness of our approach to the number of training viewpoints, as evidenced by the consistently high PSNR and SSIM metrics across different variants. This claim is further substantiated by our qualitative results in ~\cref{fig:abln_n_views}, where negligible differences are observed in the renderings, even for extreme profile views, as indicated in rows 1 and 3.

Taking into account the Landmark Distance (LD) scores, we identified that utilizing two frontal viewpoints represents the optimal training configuration for $\latentNet$. This decision stems from the fact that frontal viewpoints comprehensively cover most facial regions, allowing $\encoder$ to accurately invert these views while ensuring minimal identity loss. 

\begin{table}[ht]
\centering
\caption{\textbf{Quantitative Results: Ablation Study: Number of Viewpoints.} We report SSIM, landmarks distance (LD), and PSNR on the test data of lightstage, where  subjects are relit under novel viewpoints.} 
\begin{tabular}{lcccc}
\hline
           & SSIM $\uparrow$ & LD $\downarrow$ & PSNR $\uparrow$ \\ \hline
Views = 1  & 0.831 & 10.45 & 28.31 \\
Views = 4  & 0.834 & 10.26 & 28.30 \\
Views = 8  & 0.834 & 10.1 & 28.31 \\ \hline
Views = 2 &  \textbf{0.834} & \textbf{9.76} &\textbf{28.33} \\ \hline
\end{tabular}
\label{tab:abln_n_views}
\end{table}

\input{tex_fig/results/abln_n_views}

\paragraph{Number of Subjects: }~\label{abln_subsec_n_subjects}
We conducted an ablation study to evaluate the impact of training subject quantity on generalization performance, aiming to emphasize the benefits of integrating generative priors with supervised learning approaches. Our lightstage dataset comprises 353 subjects, and for this study, we conducted experiments with subsets of 250, 50, and 10 subjects. Our quantitative analysis revealed that the model trained with 250 subjects achieves the best performance. However, it is noteworthy that the difference in performance between this model and the one trained with as few as 10 subjects is relatively marginal. This observation, indicative of robust generalization, is further substantiated in ~\cref{fig:abln_n_subjects}. Here, we demonstrate the ability of our method to perform 3D consistent view and illumination editing on an unseen subject under various lighting conditions, as seen in rows 2 and 3.

Our observations in ~\cref{abln_subsec_n_subjects} and \cref{abln_subsec_n_views}, suggest that \OurMethod does not necessitate a densely-equipped multiview lightstage setup or extensive data collection campaigns. This advantage significantly reduces the complexities associated with hardware and data storage, thereby paving the way for more feasible and generalizable portrait relighting solutions. Such solutions could potentially be realized with minimal equipment, akin to the approach proposed by Sengupta et al.\cite{Sengupta2021ALS}, which utilizes a few desktop monitors. However, the exploration of this avenue falls outside the scope of our current project and we leave this for future work. 

\begin{table}[ht]
\centering
\caption{\textbf{Quantitative Results: Ablation Study: Number of Subjects.} We report SSIM, landmarks distance (LD), and PSNR on the test data of lightstage, where  subjects are relit under novel viewpoints.} 
\begin{tabular}{lcccc}
\hline
           & SSIM $\uparrow$ & LD $\downarrow$ & PSNR $\uparrow$ \\ \hline
Subjects = 10  & 0.829 & 10.24 & 28.26 \\
Subjects = 50  & 0.829 & 9.61 & 28.31 \\\hline
Subjects = 250 &  \textbf{0.834} & \textbf{9.76} &\textbf{28.33} \\ \hline
\end{tabular}
\label{tab:abln_n_subjects}
\end{table}
\input{tex_fig/results/abln_n_subjects}

\paragraph{Latent Editing: }
The utilization of a feedforward encoder-based inversion in our framework extends beyond merely accelerating inference. A significant advantage of this approach is that the encoded latent vector reliably remains within the latent manifold of the generator. This ablation study aims to merge the semantic manipulation capabilities inherent in the latent space with the task of relighting. It shows that our $\latentNet$ effectively operates within the rich latent manifold of EG3D. Leveraging the latent attribute directions identified by GOAE~\cite{goae2023}, we demonstrate the simultaneous editing of viewpoint and illumination alongside changes in specific facial attributes—namely, \enquote{age}, \enquote{anger}, and \enquote{glasses}. These multifaceted edits are showcased in ~\cref{fig:ablations_latent_edits}, illustrating the robust and versatile nature of our method.

\input{tex_fig/results/abln_latent_edit}
\input{tex_fig/results/supmat_challenges}
% \textbf{Different Video Source's Results}

% \subsection{Vides}

% \section{Interactive Demo}

\section{Challenges and Future Work}
While our method demonstrates effective photorealistic editing of viewpoints and relighting, there remain areas for improvement. 
\paragraph{Occlusions and non-frontal views:} Our approach depends on the pretrained 3D-aware encoder for inversion, which positions the given portrait within the canonical 3D space of the generator. However, this encoder was primarily trained on unoccluded, front-facing views. As a result, the performance of the encoder, and consequently our relighting technique, encounter challenges with non-frontal views, the presence of accessories, and occluded faces as shown in the \cref{fig:challenges}

\new{\paragraph{Hard Shadows:}To achieve relighting at interactive rates, Lite2Relight relies on relighting within the latent manifold of the generator as opposed to explicit modelling face reflectance through HDR OLAT rendering as in \cite{prao2023vorf} or explicit specular and diffuse maps as in Total Relighting~\cite{Pandey21}. Consequently currently casting hard shadows is a challenge.}

\paragraph{OLAT Synthesis:}
Furthermore, even though we use a lightstage dataset, currently, our approach does not support the synthesis of HDR (High Dynamic Range) OLAT images, restricting our ability to recreate unconventional lighting conditions. This limitation stems from the fact that OLAT images do not fall within the distribution of the pretrained generator. While training an OLAT-based generator capable of predicting a dense reflectance basis might address this issue, it lies beyond the scope of our current project. Nonetheless, exploring such a generator presents a fascinating and potentially impactful avenue for future research, promising to further advance the field of photorealistic relighting and editing.
